# Supplementary material for: Directional transport and nonlinear localization of light in a one-dimensional driven-dissipative photonic lattice
Source: arXiv:2505.11114 ancillary file (2025-05-16)
Supplement: Supplementary file 1 [file directional_transport_supp.pdf]

## I. ADDITIONAL INFORMATION ON DIRECTIONAL TRANSPORT

This section aims to provide additional information about directional emission compared to the one presented in the main paper. To quantify the directional emission in the lattice, we define the total intensities emitted to the left and right of the pumped region as

$$I_L = \sum_{m<m_{\text{pump}}} I_m; \quad I_R = \sum_{m>m_{\text{pump}}} I_m,$$

where $I_m$ denotes the normalized intensity at lattice site $m$ and $m_{\text{pump}}$ here denotes the pumped lattice sites (in this case, sites 19 and 20). The pumped sites are excluded from the summation to ensure that only the transported intensity is considered.
The directional transport ($D$) is then defined as

$$D = \frac{I_R - I_L}{I_R + I_L}.$$

By definition, $D$ lies in the range $[-1, 1]$ and provides the fraction of directional emission. $D = 0$ implies symmetric emission to both sides. Positive values of $D$ indicate net rightward transport, while negative values indicate leftward transport. Fig. 1(a) presents the numerical plot of directional transport $D$ as a function of $\Delta\phi/\pi$, while Fig. 1(b) shows the corresponding experimental results. Although experimental and simulated results show a similar overall behavior, the deviations observed in the experimental directional transport ($D$) to the numerics are due to the presence of stray light.

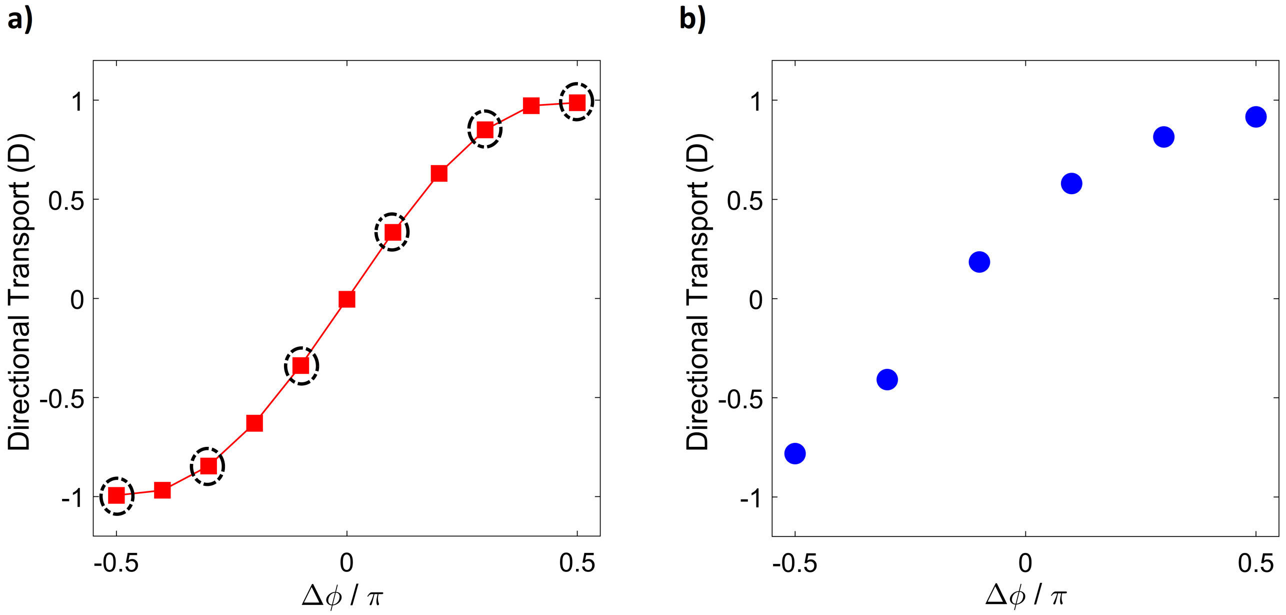


FIG. 1. Phase dependent directional transport $D(\Delta\phi)$ extracted from both numerical simulations 1(a) and experimental measurements 1(b). The six black circles in Fig. 1(a) mark the phase values used in the experimental measurements shown along the x-axis in Fig. 1(b).

To explore the emergence of directional transport, we compare the spatial intensity profiles measured experimentally and numerically. As shown in Fig. 2 and 3 (panels a–f), tuning the phase from $-0.5\pi$ to $+0.5\pi$ induces a gradual shift in the direction of light propagation within the lattice. This behavior arises from constructive and destructive interference between drive and lattice eigen modes, which alters the balance between left- and right- propagating components. Both simulations and experiments exhibit the strongest asymmetry at $\Delta\phi = \pm\frac{\pi}{2}$: a phase difference of $-\pi/2$ leads to maximum transport to the left, while $+\pi/2$ results in maximum transport to the right.

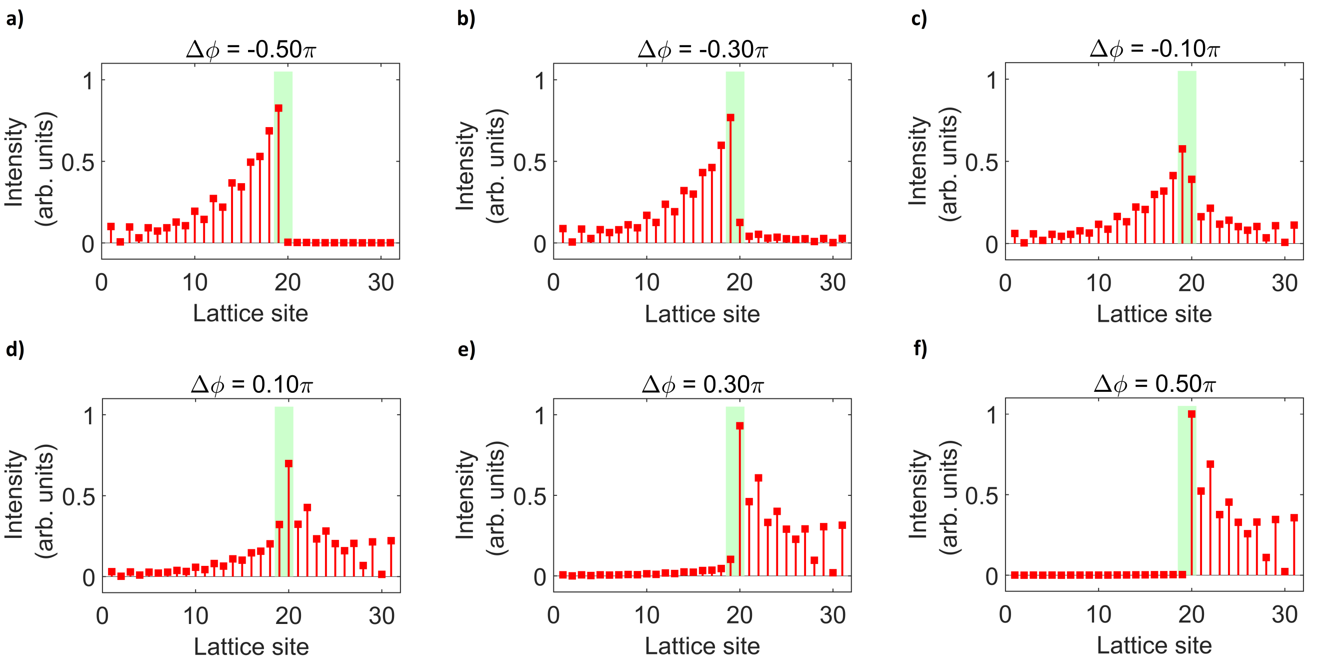


FIG. 2. (a–f) Numerical steady-state intensity profiles for different pump phase differences $\Delta\phi$ between two adjacent sites, ranging from $-0.5\pi$ to $0.5\pi$. The strongest leftward transport occurs at $\Delta\phi = -0.5\pi$, and rightward transport is maximized at $\Delta\phi = +0.5\pi$. Shaded areas correspond to the sites $(19, 20)$ where the external pump is applied.

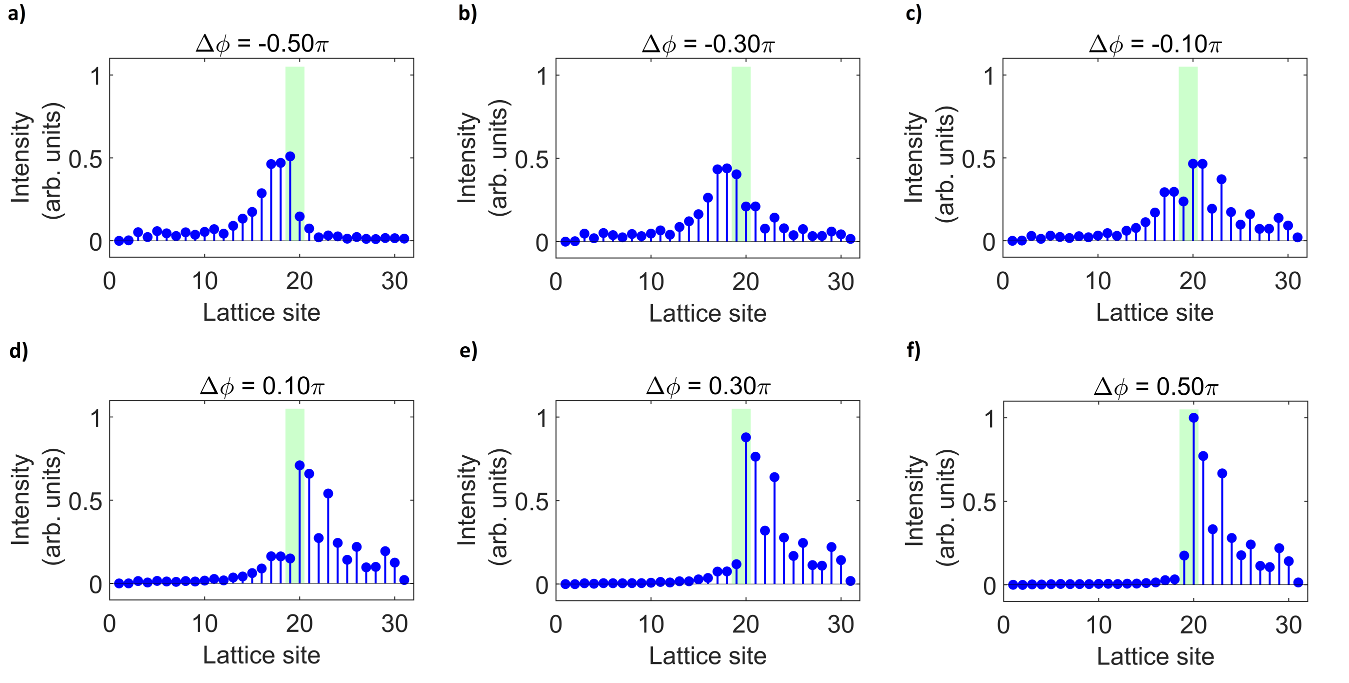


FIG. 3. (a–f) Experimentally measured intensity profiles for different pump phase differences $\Delta\phi$ between two adjacent sites, ranging from $-0.5\pi$ to $0.5\pi$. Each panel corresponds to a distinct phase difference between the two excitation spots showing qualitative agreement with the numerical results in Fig. 2. Shaded areas correspond to the sites $(19, 20)$ where the external pump is applied.

## II. ANALYTICAL DERIVATION OF SITE INTENSITY

This part aims to provide analytical results on the spatial light distribution within photonic lattices in the linear regime. To simplify the calculation without losing important physics features, we assume a polariton to be 100% photonic (and thus having no interaction) and we neglect the contribution originating from next-nearest neighbor coupling ($t' = 0$). Under these assumptions, we can write a driven-dissipative tight-binding model, in the rotating frame of the pump laser, describing the dynamics of the photon field $\psi_m$ on each site $m \in Z$:

$$i\hbar\dot{\psi}_m = (\epsilon_0 - \omega_p)\psi_m - i\gamma\psi_m - t(\psi_{m+1} + \psi_{m-1}) + F_m, \tag{1}$$

where $\epsilon_0$ is the middle band photonic energy, $\gamma$ is the radiative decay, $t$ is the nearest neighbor coupling and $F_m$ is the field source term.

It is convenient to write the problem in the reciprocal space using $\psi_m = \frac{1}{\sqrt{M}}\sum_k \psi_k e^{ikm}$ and $F_m = \frac{1}{\sqrt{M}}\sum_k F_k e^{ikm}$ to get:

$$i\hbar\dot{\psi}_k = (\epsilon_0 - \omega_p)\,\psi_k - i\gamma\psi_k - 2t\cos k\,\psi_k + F_k,$$

with $k \in [-\pi, \pi]$ and $M$ the total number of sites.

Introducing $\Delta = \omega_p - \epsilon_0$ and looking for a steady state solution, we obtain

$$\psi_k = \frac{F_k}{\Delta + 2t\cos k + i\gamma}.$$

Compared to [1], here we restrict the situation to one of interest in the main section of the paper, where only two sites $m_1$ and $m_2$ are pumped with a phase difference of $\Delta\phi$. Such pumping can be explicitly written in position space like:

$$F_m = \frac{F}{\sqrt{M}}(\delta_{m,m_1} + e^{i\Delta\phi}\delta_{m,m_2}),$$

with $\delta_{m,n}$ the Kronecker delta, or in Fourier space as:

$$F_k = \sum_m F_m e^{-ikm} = \frac{F}{\sqrt{M}}\left(e^{-ikm_1} + e^{i\Delta\phi}e^{-ikm_2}\right).$$

we can write

$$\psi_k = \frac{F}{\sqrt{M}}\frac{e^{-km_1} + e^{i\Delta\phi}e^{-ikm_2}}{\Delta + 2t\cos k + i\gamma}.$$

We transform back to real space and approximate the discrete sum in momenta by an integral to obtain

$$\psi_m = \frac{1}{\sqrt{M}}\sum_k \psi_k e^{ikm} \approx \frac{F}{2\pi}\int_{-\infty}^{\infty}\frac{e^{-ik|m-m_1|} + e^{i\Delta\phi}e^{-ik|m-m_2|}}{\Delta + 2t\cos k + i\gamma}dk, \tag{2}$$

where the integration limits have been extended from $-\infty$ to $\infty$ because the integrand vanishes outside the first Brillouin zone. This integral can be calculated using complex analysis and the residue theorem. Following the derivation as shown in Appendix B of Ref. [1], we will investigate three different scenarios and conduct the calculation explicitly in one of them to show that we obtain the same final expression, presented in the main paper. The calculations in the other scenarios are similar and present no additional complexities compared to the presented one.

The three scenarios are:

1. $m < m_1 < m_2 \Rightarrow m - m_1 < 0$ and $m - m_2 < 0$
2. $m_1 < m < m_2 \Rightarrow m - m_1 > 0$ and $m - m_2 < 0$
3. $m_1 < m_2 < m \Rightarrow m - m_1 > 0$ and $m - m_2 > 0$

**Case 1:** $m - m_1 < 0$ **and** $m - m_2 < 0$

Eq. 2 can be approximated by an integral in the limit of an infinite number of sites, and, as the integrand vanishes outside the first Brillouin zone, we can also extend the integration limits from $-\infty$ to $\infty$ to obtain

$$\psi_m \approx \frac{F}{2\pi} \int_{-\infty}^{\infty} \frac{e^{-ik|m-m_1|} + e^{i\Delta\phi} e^{-ik|m-m_2|}}{\Delta + 2t\cos k + i\gamma} dk.$$

We can solve this integral using complex integration and the residue theorem. We mainly follow what is done in the Appendix B of Ref. [1]. We provide, in the following, the different step of the calculation.

Looking for an expression for $k$ satisfying

$$\Delta + 2t\cos k \approx 0,$$

we define the resonant momentum $k_0$ through:

$$\cos k_0 = -\frac{\Delta}{2t} \quad \Rightarrow \quad k_0 = \arccos\left(-\frac{\Delta}{2t}\right).$$

Then, we expand $\cos k$ around $k = k_0$ up to first-order in $k$ to get

$$\cos k \approx \cos k_0 - \sin k_0 (k - k_0).$$

Performing some algebra by multiplying both sides by $2t$, substituting $\cos k_0$ by $-\frac{\Delta}{2t}$ and re-arranging the expression, we obtain:

$$\Delta + 2t\cos k \approx -2t \sin k_0 (k - k_0).$$

Identifying $\sin k_0$ as:

$$\sin k_0 = \sqrt{1 - \cos^2 k_0} = \sqrt{1 - \left(\frac{\Delta}{2t}\right)^2} = \frac{\sqrt{4t^2 - \Delta^2}}{2t},$$

and plugging in the previous expression, we finally get:

$$\Delta + 2t\cos k \approx -\sqrt{4t^2 - \Delta^2}(k - k_0)$$

Doing the same calculation for $k \approx -k_0$, we get:

$$\Delta + 2t\cos k \approx +\sqrt{4t^2 - \Delta^2}(k + k_0),$$

Finally, we have

$$\Delta + 2t\cos k \approx \begin{cases} -\sqrt{4t^2 - \Delta^2}\ \left[k - \arccos\left(\frac{-\Delta}{2t}\right)\right] & \text{for } k \approx k_0 \\ +\sqrt{4t^2 - \Delta^2}\ \left[k + \arccos\left(\frac{-\Delta}{2t}\right)\right] & \text{for } k \approx -k_0 \end{cases}$$

where

$$k_0 \equiv \arccos\left(\frac{-\Delta}{2t}\right),$$

Allowing us to transform Eq. (2) into

$$\psi_m \approx \frac{F}{2\pi} \int_{-\infty}^{\infty} \left[ \frac{e^{-ik|m-m_1|} + e^{i\Delta\phi} e^{-ik|m-m_2|}}{-\sqrt{4t^2 - \Delta^2}(k - k_0) + i\gamma} + \frac{e^{-ik|m-m_1|} + e^{i\Delta\phi} e^{-ik|m-m_2|}}{+\sqrt{4t^2 - \Delta^2}(k + k_0) + i\gamma} \right] dk \tag{3}$$

At this stage, it is informative to compute the density of state (DOS) to understand how it appears in the final expression. Indeed, the density of states (DOS) is defined by:

$$D(E) = \left|\frac{dk}{dE}\right| = \left|\frac{1}{\frac{dE}{dk}}\right|.$$

Starting from the dispersion relation given by:

$$E(k) = -2t\cos k \Rightarrow \frac{dE}{dk} = 2t\sin k \Rightarrow D(E) = \left|\frac{1}{2t\sin k}\right|$$

and substituting $\cos k_0 = -\frac{\Delta}{2t}$, we get:

$$\sin k_0 = \sqrt{1-\cos^2 k_0} = \frac{\sqrt{4t^2-\Delta^2}}{2t}$$

which brings

$$D(\Delta) = \frac{1}{\sqrt{4t^2-\Delta^2}}.$$

Substituting $D(\Delta)$ in Eqn. (3), we obtain

$$\psi_m \approx -\frac{FD(\Delta)}{2\pi}\int_{-\infty}^{+\infty}\left\{\underbrace{\frac{e^{-ik|m-m_1|}}{k-k_0-i\gamma D(\Delta)}}_{(1)} + \underbrace{e^{i\Delta\phi}\frac{e^{-ik|m-m_2|}}{k-k_0-i\gamma D(\Delta)}}_{(2)} - \underbrace{\frac{e^{-ik|m-m_1|}}{k+k_0+i\gamma D(\Delta)}}_{(3)} - \underbrace{e^{i\Delta\phi}\frac{e^{-ik|m-m_2|}}{k+k_0+i\gamma D(\Delta)}}_{(4)}\right\} dk$$

We can now evaluate individual integrals using the residue theorem to get an expression for $|\psi_m|^2$.

(1)

The integrand of (1) has a pole at $k = k_0 + i\gamma D(\Delta)$, which lies in the upper-half complex plane. Since $|m-m_1| > 0$, the exponential $e^{-ik|m-m_1|}$ decays as $\mathrm{Im}(k) \to -\infty$, i.e., in the lower-half plane. To ensure convergence, the contour is closed in the lower-half, which does not enclose the pole. Therefore, the integral is zero.

$$\int_{-\infty}^{+\infty} dk \frac{e^{-ik|m-m_1|}}{k-k_0-i\gamma D(\Delta)} = 0$$

(2)

Similar to the first term, the integrand of (2) has a pole at $k = k_0 + i\gamma D(\Delta)$ that lies in the upper-half plane. The exponential $e^{-ik|m-m_2|}$ decays in the lower-half, so the contour is again closed downward and the pole is not enclosed. Thus, the integral evaluates to zero.

$$\int_{-\infty}^{+\infty} dk \frac{e^{-ik|m-m_2|}}{k-k_0-i\gamma D(\Delta)} = 0$$

(3)

The integrand of (3) has a pole at $k = -k_0 - i\gamma D(\Delta)$, which lies in the lower-half plane. Since $|m-m_1| > 0$, the exponential $e^{-ik|m-m_1|}$ also decays in the lower-half. Therefore, we close the contour in the lower-half, and the pole is enclosed. The residue contributes, yielding a non-zero result ($e^{-i(-k_0-i\gamma D(\Delta))|m-m_1|} = e^{+ik_0|m-m_1|}e^{-\gamma D(\Delta)|m-m_1|}$), which brings

$$\int_{-\infty}^{+\infty} dk \frac{e^{-ik|m-m_1|}}{k+k_0+i\gamma D(\Delta)} = -2\pi i\, e^{+ik_0|m-m_1|}\, e^{-\gamma D(\Delta)|m-m_1|}$$

(4)

This term follows the same logic as the third. The integrand of (4) has a pole at $k = -k_0 - i\gamma D(\Delta)$ which lies in the lower-half plane, and the exponential decays there as well. Thus, closing the contour downward encloses the pole, and the residue contributes a non-zero value.

$$\int_{-\infty}^{+\infty} dk \frac{e^{-ik|m-m_2|}}{k+k_0+i\gamma D(\Delta)} = -2\pi i\, e^{+ik_0|m-m_2|}\, e^{-\gamma D(\Delta)|m-m_2|}$$

Thus, assembling all these results together we obtain for the field:

$$\psi_m = -FD(\Delta)i\left[e^{ik_0|m-m_1|}e^{-\gamma D(\Delta)|m-m_1|} + e^{i\Delta\phi}e^{ik_0|m-m_2|}e^{-\gamma D(\Delta)|m-m_2|}\right]$$

Taking the square modulus brings:

$$I_m = |\psi_m|^2 = |F|^2 D(\Delta)^2 \left|e^{ik_0|m-m_1|}e^{-\gamma D(\Delta)|m-m_1|} + e^{i\Delta\phi}e^{ik_0|m-m_2|}e^{-\gamma D(\Delta)|m-m_2|}\right|^2$$

We recover the equation present in the main text. In the following, we show the different cases for completeness, but we do not reproduce all the details of the calculations. We mainly explain how we recover the same expression for $I_m$.

**Case 2:** $m - m_1 > 0$ **and** $m - m_2 < 0$

Using the same derivation as in case 1, we have for Eqn. (3) in case 2:

$$\psi_m \approx -\frac{FD(\Delta)}{2\pi}\int_{-\infty}^{+\infty}\left\{\underbrace{\frac{e^{ik|m-m_1|}}{k-k_0-i\gamma D(\Delta)}}_{(1)} + \underbrace{\frac{e^{i\Delta\phi}e^{-ik|m-m_2|}}{k-k_0-i\gamma D(\Delta)}}_{(2)} - \underbrace{\frac{e^{ik|m-m_1|}}{k+k_0+i\gamma D(\Delta)}}_{(3)} - \underbrace{\frac{e^{i\Delta\phi}e^{-ik|m-m_2|}}{k+k_0+i\gamma D(\Delta)}}_{(4)}\right\}dk$$

This case is symmetric to Case 1, but the roles of $m_1$ and $m_2$ are reversed in terms of which exponential contributes. Terms (1) and (4) now contribute to the integral, while (2) and (3) vanish. The derivation proceeds in exactly the same manner, and the resulting expression for $I_m$ is unchanged.

**Case 3:** $m - m_1 > 0$ **and** $m - m_2 > 0$

Similarly, we have for Eqn. (3) in case 3:

$$\psi_m \approx -\frac{FD(\Delta)}{2\pi}\int_{-\infty}^{+\infty}\left\{\underbrace{\frac{e^{ik|m-m_1|}}{k-k_0-i\gamma D(\Delta)}}_{(1)} + \underbrace{\frac{e^{i\Delta\phi}e^{ik|m-m_2|}}{k-k_0-i\gamma D(\Delta)}}_{(2)} - \underbrace{\frac{e^{ik|m-m_1|}}{k+k_0+i\gamma D(\Delta)}}_{(3)} - \underbrace{\frac{e^{i\Delta\phi}e^{ik|m-m_2|}}{k+k_0+i\gamma D(\Delta)}}_{(4)}\right\}dk$$

In this case, both exponential terms $e^{ik|m-m_1|}$ and $e^{ik|m-m_2|}$ decay in the upper-half complex plane. As a result, the contour is closed in the upper-half, enclosing the poles at $k = k_0 + i\gamma D(\Delta)$. The poles of the first two terms lie in the upper-half plane and are enclosed. Therefore, only the contributions from terms (1) and (2) yield non-zero

residues. After applying the residue theorem, we again obtain the same structure for $\psi_m$, and consequently the same final expression for the intensity $I_m = |\psi_m|^2$.

Therefore, in all three cases, we get the following result;

$$I_m = |\psi_m|^2 = |F|^2 D(\Delta)^2 \left| e^{ik_0|m-m_1|} e^{-\gamma D(\Delta)|m-m_1|} + e^{i\Delta\phi} e^{ik_0|m-m_2|} e^{-\gamma D(\Delta)|m-m_2|} \right|^2 \quad (4)$$

### A. Derivation of the criteria for directionality

To derive the conditions under which directional emission occurs, we analyze the steady-state intensity in the region to the left of both pump sites, i.e., for $m < m_1$ and $m < m_2$. The link with the general expression is made by having in mind that $(m - m_1) = -|m - m_1|$ and $(m - m_2) = -|m - m_2|$. Identifying the conditions for complete destructive interference, we can determine the values of $\Delta\phi$ and $k_0$ that suppress propagation in this direction and thus lead to directional transport. Specifically, the intensity at the site $m$ takes the form:

$$I_m = |F|^2 D(\Delta)^2 \underbrace{\left| e^{-ik_0(m-m_1)} e^{\gamma D(\Delta)(m-m_1)} + e^{i\Delta\phi} e^{-ik_0(m-m_2)} e^{\gamma D(\Delta)(m-m_2)} \right|^2}_{0 \text{ (complete destructive interference)}}$$

$$I_m = |F|^2 D(\Delta)^2 |A + B|^2 = |F|^2 D(\Delta)^2 (|A|^2 + |B|^2 + A^*B + AB^*)$$

$$A = e^{-ik_0(m-m_1)} e^{\gamma D(\Delta)(m-m_1)}$$
$$B = e^{i\Delta\phi} e^{-ik_0(m-m_2)} e^{\gamma D(\Delta)(m-m_2)}$$

$$|A|^2 = e^{2\gamma D(\Delta)(m-m_1)}$$
$$|B|^2 = e^{2\gamma D(\Delta)(m-m_2)}$$
$$A^*B = e^{i\Delta\phi} e^{ik_0(m_2-m_1)} e^{\gamma D(\Delta)(2m-m_1-m_2)}$$
$$AB^* = e^{-i\Delta\phi} e^{-ik_0(m_2-m_1)} e^{\gamma D(\Delta)(2m-m_1-m_2)}$$

$$I_m/(|F|^2 D(\Delta)^2) = e^{2\gamma D(\Delta)(m-m_1)} + e^{2\gamma D(\Delta)(m-m_2)} + e^{\gamma D(\Delta)(2m-m_1-m_2)} \left[2\cos\left(\Delta\phi + k_0(m_2 - m_1)\right)\right]$$

In the limit of small $\gamma$ compared to $t|m_1 - m_2|$, we have $e^{-\gamma D(\Delta)|m-m_2|} \approx e^{-\gamma D(\Delta)|m-m_1|}$ allowing us to write

$$I_m/(|F|^2 D(\Delta)^2) \approx 2e^{2\gamma D(\Delta)(m-m_1)} \left[1 + \cos\left(\Delta\phi + k_0(m_2 - m_1)\right)\right],$$

which is equal to 0 in the case where

$$\Delta\phi + k_0(m_2 - m_1) = (2\ell + 1)\pi, \quad \ell \in \mathbb{Z}.$$

### B. Derivation of the criteria for linear localization

To analytically investigate the conditions under which localization arises in Eqn. (4), we consider the steady-state field amplitude at an arbitrary site $m$ resulting from coherent driving at two sites $m_1$ and $m_2$. In the limit of small $\gamma$ compared to $t|m_1 - m_2|$, we have $e^{-\gamma D(\Delta)|m-m_2|} \approx e^{-\gamma D(\Delta)|m-m_1|}$, allowing us to write the field as

$$\psi_m = FD(\Delta)e^{-\gamma D(\Delta)|m-m_2|}\left[e^{ik_0|m-m_1|} + e^{i\Delta\phi}e^{ik_0|m-m_2|}\right]. \tag{5}$$

We want to identify how constructive or destructive interference between the two driving fields can lead to enhanced localization at specific sites, depending on the pump separation and relative phase. We aim to find conditions on $\Delta\phi$ and $k_0$ such that:

1. Destructive interference occurs at all sites $m \leq m_1$,
2. Destructive interference occurs at all sites $m \geq m_2$,

#### 1. Destructive Interference for $m \leq m_1$

Introducing $p \geq 0$ such that $m = m_1 - p$ we have:

$$|m - m_1| = p, \quad |m - m_2| = d + p, \quad \text{where } d = m_2 - m_1$$

$$\psi_m = FD(\Delta)e^{-\gamma D(\Delta)|m-m_2|}e^{ik_0 p}\left(1 + e^{i(\Delta\phi + k_0 d)}\right)$$

Destructive interference conditions requires $\psi_m = 0$ which is satisfied for:

$$\boxed{1 + e^{i(\Delta\phi + k_0 d)} = 0} \tag{6}$$

#### 2. Destructive Interference for $m \geq m_2$

Introducing $p_2 \geq 0$ such that $m = m_2 + p_2$ we have:

$$|m - m_1| = d + p_2, \quad |m - m_2| = p_2$$

$$\psi_m = FD(\Delta)e^{-\gamma D(\Delta)|m-m_2|}e^{ik_0(d+p_2)}\left(1 + e^{i(\Delta\phi - k_0 d)}\right)$$

Destructive interference conditions requires $\psi_m = 0$ which is satisfied for:

$$\boxed{1 + e^{i(\Delta\phi - k_0 d)} = 0} \tag{7}$$

Assembling these conditions of Eqn. (6) and (7) require simultaneously satisfying:

$$\Delta\phi = (2n+1)\pi + k_0 d \tag{i}$$
$$\Delta\phi = (2n+1)\pi - k_0 d, \tag{ii}$$

As $\Delta\phi$ is defined modulo $2\pi$, the only solution is $k_0 d = \pm\pi$. Knowing that $d = 2$, it follows that $k_0$ has to be equal to $\pm\frac{\pi}{2}$. These $k_0$ values are satisfied only for a detuning $\Delta = 0$, providing the condition to observe localization.

## III. EFFECT OF DISORDER IN NUMERICAL SIMULATION

To study the effects of disorder in both onsite and hopping, we performed numerical simulations over multiple random disorder configurations. For each value of disorder strength $\alpha$, the system was simulated with 25 independent disorder realizations. At each realization, the steady-state intensity profile was extracted and normalized. The resulting spatial profiles were then averaged to obtain the disorder-averaged intensity distribution. The error bars represent the standard deviation of the intensity at each site across these 25 realizations, indicating the spread due to random disorder.

### A. Onsite Disorder

The on-site disorder for $i \in \{\text{photon}, \text{exciton}\}$ is given by:

$$\text{onsite\_disorder}_i = \alpha \cdot t_1^{(0)} \cdot [\text{rand}(1, N_{\text{pillars}}) - 0.5]$$

where $\alpha$ is the disorder strength, $t_1^{(0)}$ is the unperturbed nearest hopping and $\text{rand}(1, N_{\text{pillars}})$ generates a random array of values uniformly distributed in the interval $[0, 1]$. The subtraction of 0.5 centers the disorder around zero.

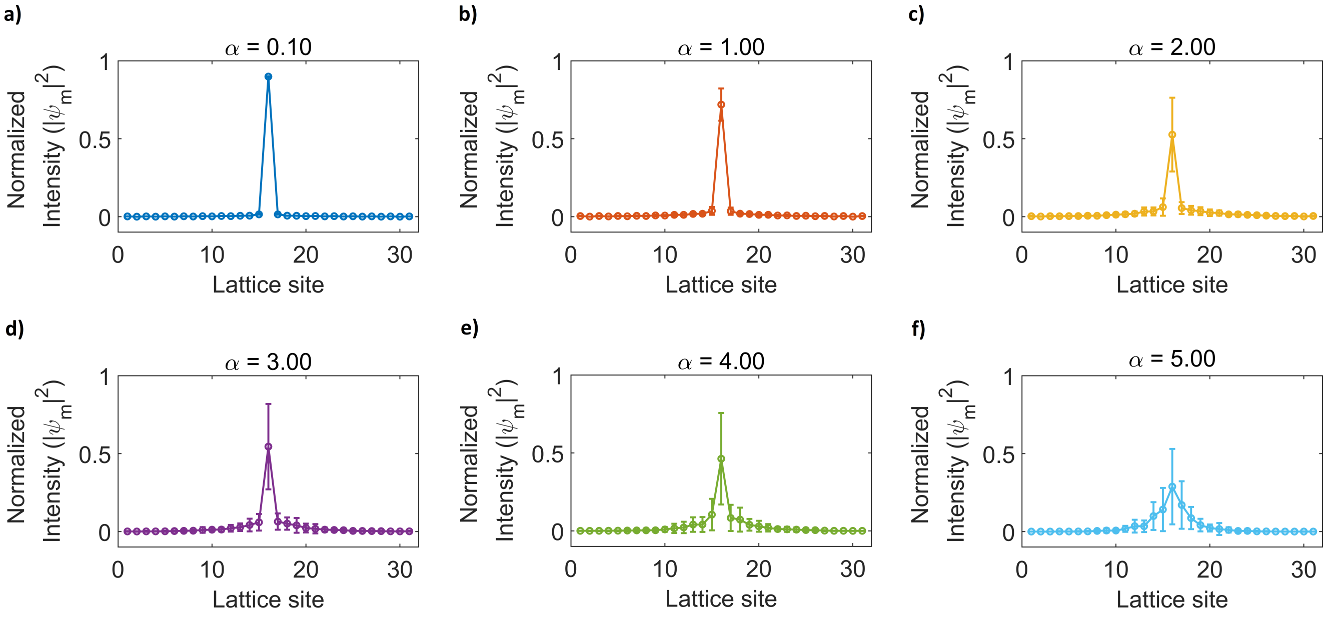


FIG. 4. Normalized intensity profiles for increasing onsite disorder strength $\alpha$. (a)–(f) correspond to: (a) $\alpha = 0.1$, (b) $\alpha = 1$,(c) $\alpha = 2$, (d) $\alpha = 3$, (e) $\alpha = 4$ and (f) $\alpha = 5$.

### B. Hopping Disorder

The hopping disorder for the nearest-neighbor ($t_1$, $t_2$) and next-nearest-neighbor ($t_{\text{NNN}}$) couplings is introduced as:

$$\begin{aligned} t_1^{\text{disorder}} &= t_1^{(0)} + \alpha \cdot t_1^{(0)} \cdot [\text{rand}(1, N_{\text{pillars}} - 1) - 0.5] \\ t_2^{\text{disorder}} &= t_2^{(0)} + \alpha \cdot t_2^{(0)} \cdot [\text{rand}(1, N_{\text{pillars}} - 1) - 0.5] \\ t_{\text{NNN}}^{\text{disorder}} &= t_{\text{NNN}}^{(0)} + \alpha \cdot |t_{\text{NNN}}^{(0)}| \cdot [\text{rand}(1, N_{\text{pillars}} - 2) - 0.5] \end{aligned}$$

where $t_1^{(0)}, t_2^{(0)}, t_{\text{NNN}}^{(0)}$ are the unperturbed hopping amplitudes, $\alpha$ is the disorder strength (same as for the on-site disorder), $\text{rand}(1, N)$ generates a uniformly distributed random array in $[0, 1]$.

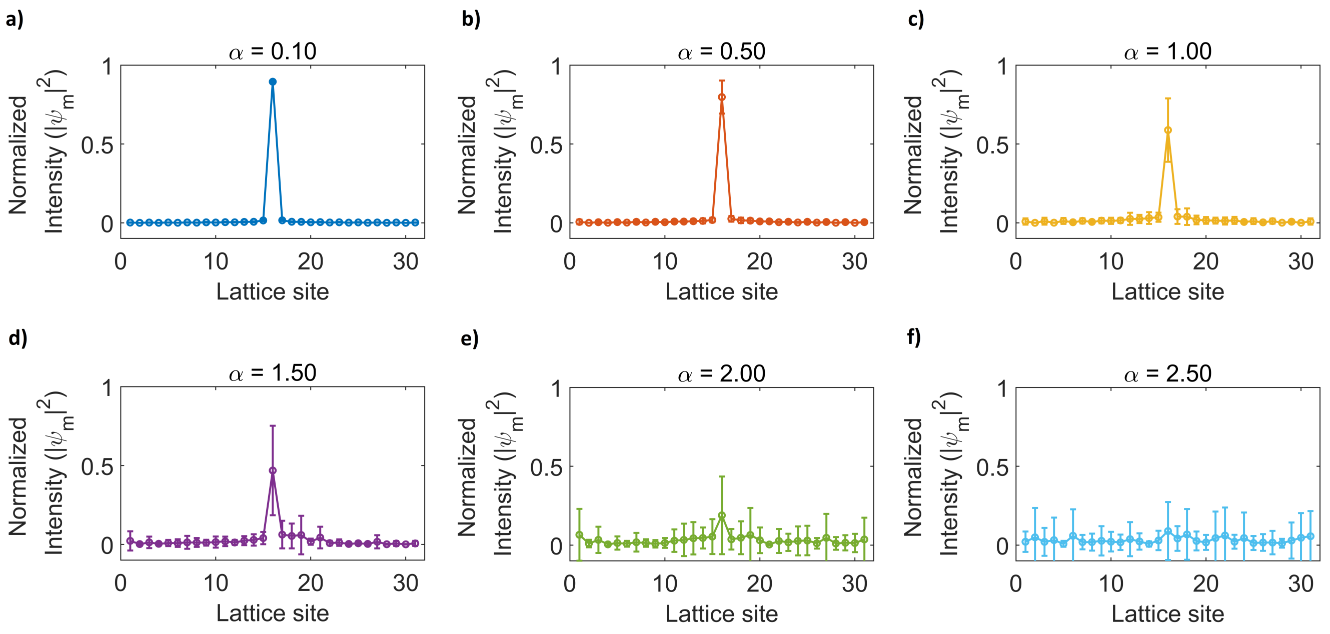


FIG. 5. Normalized intensity profiles for increasing hopping disorder strength $\alpha$. (a)–(f) correspond to: (a) $\alpha = 0.1$, (b) $\alpha = 0.5$,(c) $\alpha = 1$, (d) $\alpha = 1.5$, (e) $\alpha = 2$ and (f) $\alpha = 2.5$.

[1] A. Muñoz de las Heras, A. Amo, and A. González-Tudela, Nonlinearity-enabled localization in driven-dissipative photonic lattices, Phys. Rev. A **109**, 063523 (2024).
